# Supplementary material for: How much better are InGaN/GaN nanodisks than quantum wells - oscillator strength enhancement and changes in optical properties
Source: arXiv:1309.6264 source file (2014-01-22)
Supplement: Supplementary file 1 [file Supplementary_Materials.pdf]

# Supplementary material for: How much better are InGaN/GaN nanodisks than quantum wells – oscillator strength enhancement and changes in optical properties

Lei Zhang,[1] Leung-Kway Lee,[2] Chu-Hsiang Teng,[2] Tyler A. Hill,[1] Pei-Cheng Ku,[2] and Hui Deng[1, a)]

[1)]*Department of Physics, University of Michigan, 450 Church Street, Ann Arbor, MI 48109, USA*

[2)]*Department of Electrical Engineering and Computer Science, University of Michigan, 1301 Beal Ave., Ann Arbor, MI 48109, USA*

(Dated: 13 January 2014)

[a)]Electronic mail: Correspondence should be sent to dengh@umich.edu regarding optical measurements and to peicheng@umich.edu regarding materials synthesis.

## CONTENTS


**I. Strain and exciton potential profiles in a nanodisk** 2

**II. External optical effects** 6

A. Absorption efficiency $\eta_{abs}$ 6

B. The local density of photon states factor $F_p$ and collection efficiency $\eta_{col}$ 7

C. Methods to improve $F_p$ 10

**References** 11


## I. STRAIN AND EXCITON POTENTIAL PROFILES IN A NANODISK

In this section, we derive the Equ. 1 in the main text and the potential profile of exciton in a strained InGaN nanodisk (ND), based on a simple phenomenological model of 2D coupled-springs (Fig. S1(a)).

We will show below that the exciton potential profile $E(r, D)$ at the radial position $r$ of a ND of diameter $D$ is given by:

$$E(r, D) = E_0 - B_m[1 - \text{sech}(\kappa D/2)\cosh(\kappa r)], \tag{S1}$$

in which, $E_0$ corresponds to the exciton energy of a fully strain-relaxed InGaN ND, in the limit of $D = 0$ nm; $B_m$ corresponds to the maximum energy shift in a fully-strained InGaN ND at a given excitation intensity $P$, in the limit of $D \to \infty$; and $1/\kappa$ corresponds to the length scale where strain relaxation and fast increase of the bandgap energy occurs. The dependence of $E(r = 0, D)$ on $D$ reflects the experimentally measured photoluminescence (PL) energy $E$ vs. $D$ in Fig. 2(a) in the main text, as given by the Equ. 1 in the main text and reproduced below:

$$E(D) = E_0 - B_m[1 - \text{sech}(\kappa D/2)]. \tag{S2}$$

The purpose of this model is *NOT* to provide a method to rigorously calculate the $E$, which could be done using sophisticated 3D simulation packages[1] based on $k{\cdot}p$ method considering spontaneous polarization and strain-induced deformation and piezo-electric polarization potentials[2]. The purpose of this model is to provide a way to extract, directly from experimental data, the key parameters, $E_0$, $B_m$ and $\kappa$, which characterize the strain relaxation in our NDs. In addition, unlike

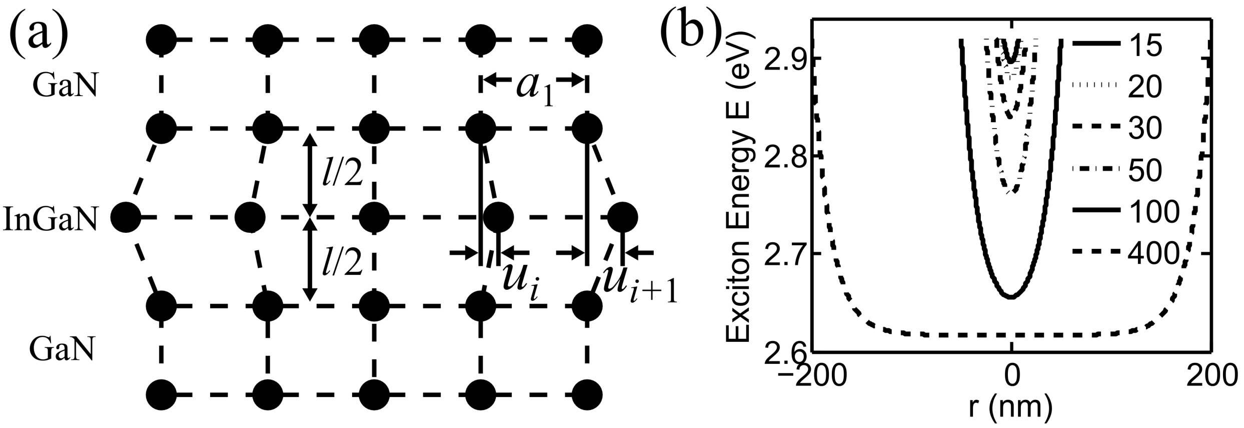


FIG. S1. (a) The schematic plot of the simple 1D theory described in the text. (b) The exciton potential profile at $P = 0.4$ W/cm$^2$ along the lateral direction in NDs with $D = 15, 20, 30, 50, 100, 400$ nm, plotted using the fitting results of Fig. 2(a), $E_0 = 2.92$ eV, $B_m(P = 0.4) = 303$ meV and $\kappa = 0.055$ nm$^{-1}$.

$k \cdot p$ simulation packages, this model does not rely on the choice of material constants, some of which are often controversial, some are not even available for low temperatures[3].

We illustrate our model in Fig. S1(a). The InGaN quantum well (QW) of thickness $l$ is simplified to a single layer of 1D lattice, $l/2$ away from the upper and lower GaN barriers. Black dots represent the lattice sites. The upper and lower lattices represent the GaN barriers. The lattice constants of GaN and InGaN perpendicular to the $c$-axis are $a_1$ and $a_2$, respectively. If the InGaN layer is fully stressed, the InGaN lattice lines up with the GaN lattices and has lattice constance $a_1$. This represents the limit of infinite lateral size, which we call the pre-relaxation configuration. Due to the finite lateral size of our ND the strain is partially relaxed to minimize the mechanical elastic energy $E_m$ of the entire system, which we call the post-relaxation configuration. We assume that the GaN lattices are fixed for simplicity. Note that this will lead to an overestimation of the change in the piezo-electric polarization fields, since tensile-strained GaN will produce opposite polarization charges at the InGaN/GaN interfaces. But this will be taken into account by the magnitude of the $B_m$ factor. The displacement of the $i^{\text{th}}$ lattice site in the post-relaxation configuration in respect to the pre-relaxation configuration is denoted as $u_i$.

The equilibrium value of $u_i$ is determined by both minimization of the total elastic energy $E_m$ and the balance between forces at each site $i$. At each site, the atom is subject to a shear stress $F_{si}$ between InGaN and GaN layers and a hydrostatic stress $F_{hi}$ within the InGaN layer. The two

forces are given by the displacement $u_i$ as:

$$F_{si} = -k_1 u_i, F_{hi} = k_2(u_{i-1} + u_{i+1} - 2u_i). \tag{S3}$$

The coefficients $k_1$ and $k_2$ can be understood as related to the Shear modulus at the InGaN/GaN interface and the Young's modulus in InGaN QW layer, respectively. Local force balance requires that:

$$F_{si} + F_{hi} = 0. \tag{S4}$$

Substituting Equ. S3 into Equ. S4, and translating into the continuous form yields:

$$k_1 u = k_2 a_1^2 \frac{\mathrm{d}^2 u}{\mathrm{d}r^2}, \tag{S5}$$

in which $r$ is the radial distance from the center of the InGaN disk. This equation can be readily solved considering that $u(r = 0) = 0$ at the center of the disk and that $u(r)$ is an odd function of $r$, resulting in:

$$u(r) = C\left(e^{\kappa r} - e^{-\kappa r}\right), \kappa = \frac{1}{a_1}\sqrt{\frac{k_1}{k_2}}. \tag{S6}$$

Here $C$ is a constant to be determined.

The total elastic energy $E_m$ of the InGaN lattice, ignoring the coupling energy between the InGaN lattice and the barrier layers, can be written as:

$$E_m = \sum_i \frac{1}{2}k_1 u_i^2 + \frac{1}{2}k_2[(a_2 - a_1) - (u_i - u_{i-1})]^2. \tag{S7}$$

Re-writing $E_m$ in the continuous form gives:

$$\begin{aligned} E_m &= 2\int_0^{D/2} \frac{1}{2a_1}[k_1 u^2 + k_2 a_1^2 \left(\frac{a_2 - a_1}{a_1} - \frac{\mathrm{d}u}{\mathrm{d}r}\right)^2]\mathrm{d}r \\ &= 2\sqrt{k_1 k_2}\sinh\left(2\kappa D/2\right)C^2 + 4k_2(a_1 - a_2)\sinh\left(\kappa D/2\right)C + \frac{(a_1 - a_2)^2}{a_1}k_2 D/2. \end{aligned} \tag{S8}$$

Minimizing $E_m$ above gives $C$ and thus $u(r)$ as:

$$C = \frac{a_2 - a_1}{2}\sqrt{\frac{k_2}{k_1}}\mathrm{sech}\left(\kappa D/2\right), \tag{S9}$$

$$u(r) = (a_2 - a_1)\sqrt{\frac{k_2}{k_1}}\mathrm{sech}\left(\kappa D/2\right)\sinh\left(\kappa r\right). \tag{S10}$$

With $u(r)$, we obtain the hydrostatic compression strain along the radius direction defined as:

$$\varepsilon(r) = -\frac{a_2 - a_1}{a_1} + \frac{du}{dr} = \varepsilon_0\left[1 - \mathrm{sech}\left(\kappa D/2\right)\cosh\left(\kappa r\right)\right], \tag{S11}$$

in which $\varepsilon_0 = -(a_2 - a_1)/a_1$ denotes the maximum strain in a fully stressed InGaN layer.

Finally, since the shift of the InGaN bandgap due to the piezo-electric field intensity is proportional to $\varepsilon$, we obtain the potential profile given in Equ. S1 and the PL energy dependence on $D$ given in Equ. S2. For simplicity, we take into account the effect of screening by treating $B_m$ as a function of $P$, while having $E_0$ and $\kappa$ being independent on $P$. Obviously, $B_m(P)$ decreases as $P$ increases as reflected by the data in Fig. 2(a) in the main text.

The parameters, $E_0$, $B_m$ and $\kappa$, can be extracted directly from the $E$ vs. $D$ data in Fig. 2(a): $E_0 = 2.92$ eV, $B_m(P = 0.4) = 303$ meV, $B_m(P = 14) = 19$ meV and $\kappa = 0.055$ nm$^{-1}$. Using the $\kappa$ value, we estimated the length scale of strain relaxation from the sidewall as $R_{\text{relax}} \sim 1/\kappa =$ 18 nm, consistent with previous studies.[4]

Using the fitted parameters, we can obtain the potential profile of exciton. Fig. S1(b) shows $E(r, D)$ vs. $r$ at $P = 0.4$ W/cm$^2$ for InGaN NDs of $D = 15$, 20, 30, 50, 100, and 400 nm. The uneven strain relaxation along the radial direction leads to an effective confinement potential for the exciton. This confinement potential serves as a barrier that hinders excitons from fast surface recombination and, therefore, may have important impacts on carrier dynamics in our NDs, especially those in the quantum dot (QD) limit[5].

Note that due to the random fluctuations in the indium-fraction of $< 2\%$ and in the QW thickness of about 2 monolayers across the InGaN layer, there is inevitably an inhomogeneous broadening in the PL energy $E$ of NDs. This broadening is further enhanced if there exist strong polarization fields. Therefore, smaller NDs will have less broadening compared to larger ones due to strain relaxation. At low excitation intensities, only the lowest states are filled with carriers and emit light. Therefore, the measured $E$ data, hence the fitted parameters using the model, effectively corresponds to a sample with slightly higher indium fraction or slightly thicker QW thickness or both.

The main limitation of the model is that it does not include the contribution of spontaneous polarization to the potential profile $E(r, D)$. The spontaneous polarization field has the opposite sign as the piezo-polariton field but is much smaller in magnitude when significant strain exists. Hence it modifies $E(r, D)$ mainly near the side wall, where the strain relaxation greatly reduces the piezo-polarization but does not affect the spontaneous polarization.[3] However, if a ND's diameter is so small that the spontaneous polarization is stronger than the piezo-polarization, the expression of $E(r, D)$ will significantly deviate from Equ. S1. In this case, further reduction of the piezo-polarization will lead to an increase in the magnitude of the overall polarization and, thus, an

decrease in $E$. However, this is not obvious for Fig. 2(a) in the main text, suggesting that the Equ. S1 is still approximately valid even in the smallest NDs investigated here.

## II. EXTERNAL OPTICAL EFFECTS

At a given excitation laser intensity, the measured $I$, the PL intensity per unit area, of an InGaN ND is determined by the excitation intensity $P$, light absorption efficiency $\eta_{abs}$ of the nanopillar, internal quantum efficiency (IQE) $\eta_{int}$, and the output light collection efficiency $\eta_{col}$ as:

$$I \propto P\eta_{abs}\eta_{int}\eta_{col}. \tag{S12}$$

The IQE $\eta_{int}$ can be calculated as the ratio between the radiative decay rate $\gamma_r$ and the total decay rate $\gamma_{tot}$:

$$\eta_{int} = \gamma_r/\gamma_{tot}. \tag{S13}$$

At the presence of nonradiative decay, $\eta_{int}$ is enhanced by the increase of $\gamma_r$, which is proportional to both the exciton oscillator strength $f_{os}$ and the local density of photon states (LDPS) factor $F_p$. In this section we calculate the $\eta_{abs}$, $F_p$ and $\eta_{col}$ using finite-difference-time-domain (FDTD) method with the commercial software Lumerical. Using the simulation results we can extract the diameter $D$ dependence of $\eta_{int}$, $\gamma_r$ and $f_{os}$ from the measured $I$ and $\gamma_{tot}$ vs. $D$ data, as described in the main text.

### A. Absorption efficiency $\eta_{abs}$

In the experiment, we used a 390 nm (3.18 eV) pulsed laser to excite the sample at $\theta = 55^\circ$ from the normal direction (Fig. S2(a)). We neglect the absorption of the incident light by GaN, due to its large bandgap of $\sim$ 3.5 eV. To calculate the absorption in the InGaN layer, we first calculated the spatial distribution of the optical field $\vec{E}(x, y, z)$ produced by an incident plane wave. The average absorption efficiency $\overline{\eta_{abs}}$ can then be calculated via:

$$\overline{\eta_{abs}} = \frac{4}{\pi D^2 l}\int_{ND} -\frac{1}{2}\omega\epsilon_0|\vec{E}|^2\mathrm{Im}(\epsilon)\mathrm{d}V, \tag{S14}$$

in which $\omega = 2\pi/\lambda$ is the angular frequency of the excitation laser, $\epsilon_0$ is the vacuum permittivity, $\mathrm{Im}(\epsilon)$ is the imaginary part of the dielectric constant $\epsilon$, $D$ and $l$ are the diameter and thickness of

the InGaN ND, respectively. The integration only covers the ND region. Since $\epsilon$ is constant in the InGaN ND, we have:

$$\overline{\eta_{abs}} \propto \frac{1}{D^2} \int_{ND} |\vec{E}|^2 \mathrm{d}V. \tag{S15}$$

The exact $\epsilon$ of $In_{0.15}Ga_{0.85}N$ is not known. Hence we approximate it using the $\epsilon$ of bulk GaN. This is approximately valid, since our InGaN NDs have a small thickness (3 nm) and a low indium composition ($\sim$ 15%), which should not disturb the $\vec{E}(x, y, z)$ of a pure GaN nanopillar too much. We verified this by assigning the extinction coefficient $k$ of the InGaN ND to be 0.5, based on the $k$ values of bulk GaN and InN[6], and got the same trend as that shown in Fig. 3(a) in the main text after FDTD simulation.

As shown in Fig. 3(a) in the main text, the absorption efficiency $\overline{\eta_{abs}}$ is almost the same for very small ($D < 40$ nm) and very large ($D > 1000$ nm) NDs. However, it is enhanced by up to five times for NDs of diameter 100–200 nm. Fig. S2(b-d) compared the 2D cross sections of $|\vec{E}(x, y, z)|^2$ for NDs of diameters $D = 10$ nm, 160 nm and 1000 nm, respectively. At $D = 160$ nm, the nanopillar effectively forms a low-quality cavity; while at $D = 10$ nm and 1000 nm, coupling of the incident light into the nanopillar is poor.

## B. The local density of photon states factor $F_p$ and collection efficiency $\eta_{col}$

The local density of photon states (LDPS) factor $F_p$ in this work is defined as the ratio of LDPS $\rho$ of a dipole in the GaN nanopillar to that of the same dipole in bulk GaN. Numerically, this can be calculated using the ratio of the radiation powers of the two cases[7]. The first-lens collection efficiency $\eta_{col}$ is defined by the ratio of the far-field radiation power within a collection cone of NA= 0.6 (Fig. S3(a)) vs. the total radiation power. In the simulation, we used a wavelength $\lambda = 420$ nm, corresponding to the PL energy of NDs. Both quantities $F_p(\vec{p}, r; D)$ and $\eta_{col}(\vec{p}, r; D)$ depend on the diameter $D$ of the ND, radial position $\vec{r}$ of the dipole and polarization $\vec{p}$ of the dipole. We define tangential polarization $\vec{p} \perp \vec{r}$ as $\vec{p}_{\perp}$ and radial polarization $\vec{p} \parallel \vec{r}$ as $\vec{p}_{\parallel}$ (Fig. S3(b)). The electromagnetic field generated by a randomly oriented dipole can be obtained exactly from the fields generated by a tangential and a radial dipole, due to the vectorial nature of the electromagnetic field.

Fig. S3(c) shows that the $F_p$ generally increases with $D$ for dipoles of both polarizations. In small NDs of $D < 40$ nm, from $r = 0$ to $D/2$, the $F_p$ only increase slightly. In large NDs of $D > 100$ nm, from $r = 0$ to $D/2$, the $F_p$ is nearly constant until $r$ is within $\sim$ 50 nm from $D/2$.

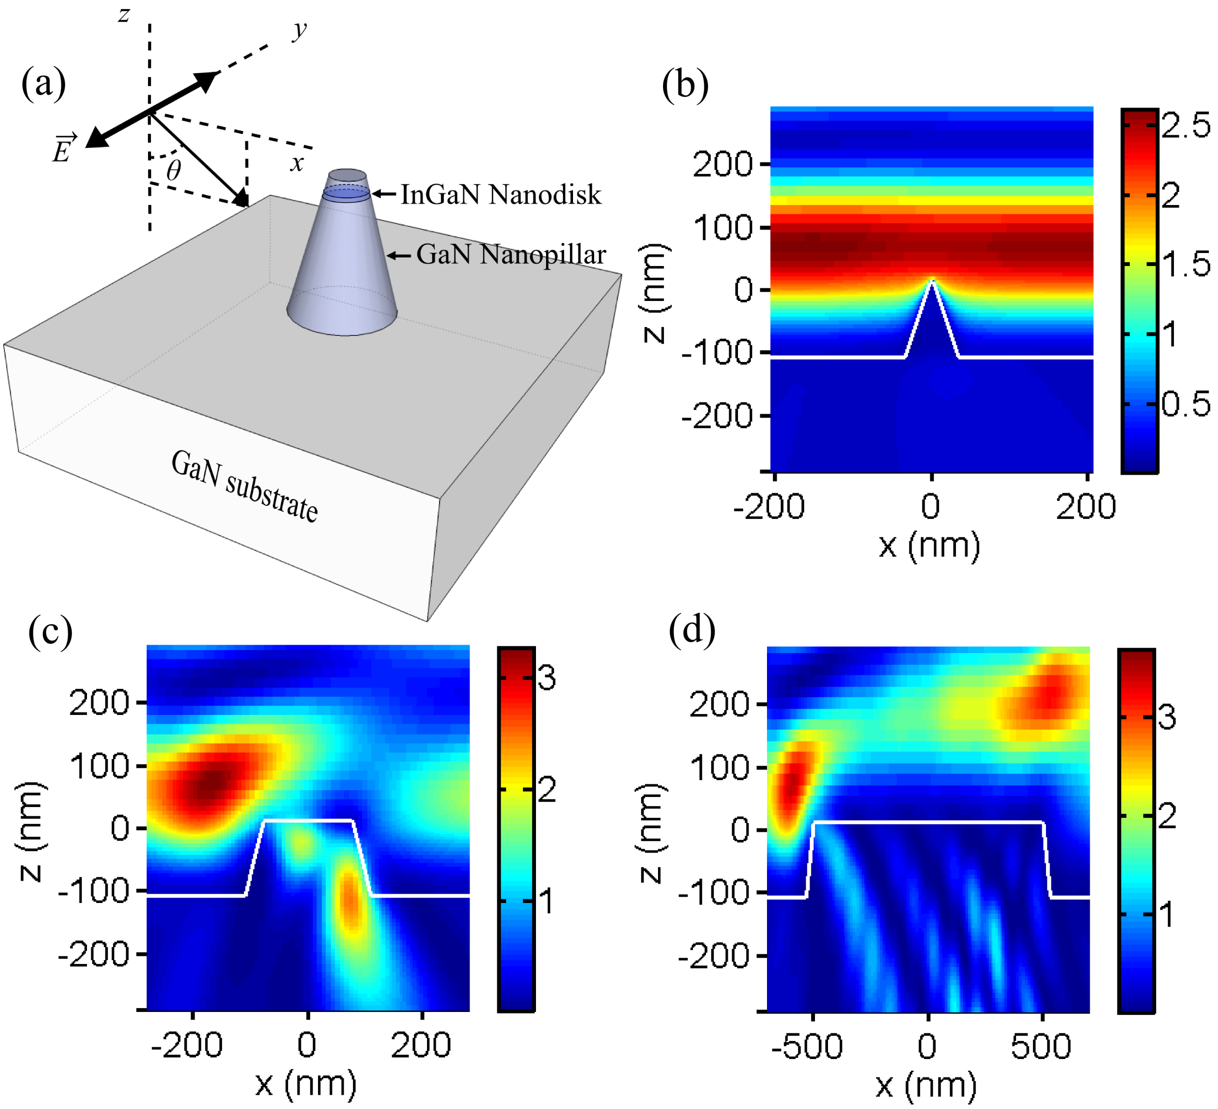


FIG. S2. (a) Schematic plot of the incidence of a plane wave to a InGaN ND in a GaN nanopillar. The propagation direction of the incident light is $\theta = 55°$ apart from the normal direction, $z$-axis. The polarization is along the $y$-axis. The nanopillar has a height of 120 nm and a sidewall angle of 75°. The center of the ND is 11.5 nm beneath the top cone surface. (b-d) $xz$-plane 2D cross section maps of $|\vec{E}(x, y, z)|^2$ for a 390 nm plane wave coupling to NDs of diameters $D$ = 10 nm, 160 nm and 1000 nm, respectively. The white lines outline the nanopillar.

Close to $r = D/2$, $F_p(\vec{p}_\perp)$ fluctuates by $< 20\%$ and $F_p(\vec{p}_\parallel)$ decreases by $\sim 8$ folds. In NDs of 40 nm $< D <$ 100 nm, both $F_p(\vec{p}_\perp)$ and $F_p(\vec{p}_\parallel)$ drops significantly as $r$ approaches $D/2$, but the decrease is not as drastic as that of $F_p(\vec{p}_\parallel)$ in larger NDs.

The $F_p$ behavior can be understood using the results of earlier studies on the spontaneous emission of a dipole placed closely to the interface of two infinite dielectric materials with refractive

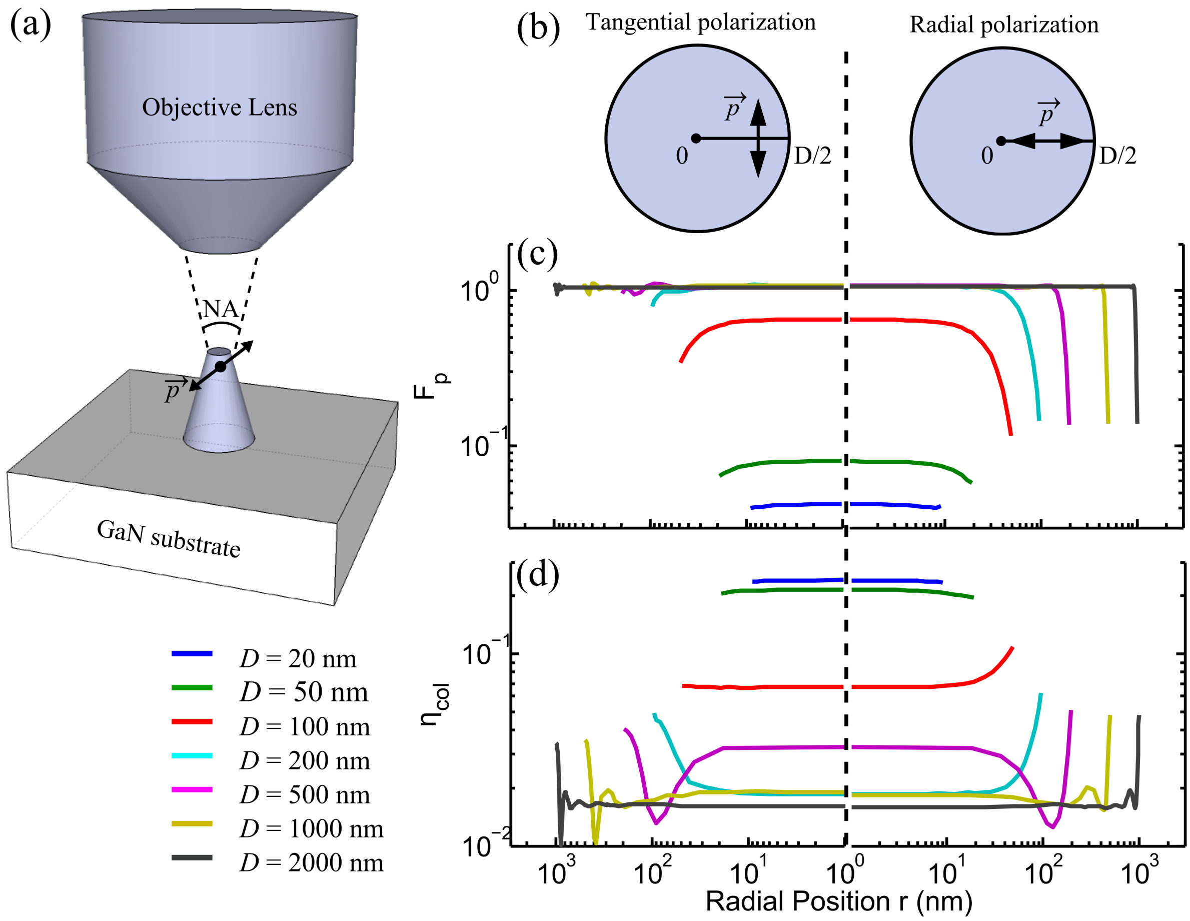


FIG. S3. (a) Schematic plot of the dipole in the nanopillar and the first-lens collection. (b) The definition of tangential dipole and radial dipole. (c-d) The $F_p$ and $\eta_{col}$ for tangential (left column) and radial (right column) dipoles at different radial positions $r$. Different line colors represents different ND diameters.

indices $n = n_1$ and $n_2$, respectively[8,9]. Considering the case in which $n_1 > n_2$, as the dipole approaches the interface to within half of the wavelength from the side of $n = n_1$, if its polarization is parallel to the interface, the $F_p$ will oscillate mildly; if its polarization is perpendicular to the interface, the $F_p$ will decrease quickly toward a finite value. This explains well the $F_p$ behavior for dipoles in NDs of $D > 100$ nm. In smaller NDs, the dipole is always close to the sidewall air-dielectic interface, so its $F_p$ is always a small but finite value.

Fig. S3(d) shows that the $\eta_{col}$ generally decreases with $D$ for dipoles of both polarizations. Unlike $F_p$, the behavior of $\eta_{col}$ is largely insensitive to the dipole's polarization. In small NDs of $D < 40$ nm, $\eta_{col}$ is nearly constant with $\eta_{col}(r = 0)$ slightly greater than $\eta_{col}(r = D/2)$. In large NDs of $D > 500$ nm, the $\eta_{col}$ in the region $D/2 - 100$ nm $< r < D/2$ is two to three times of that in the rest of the ND.

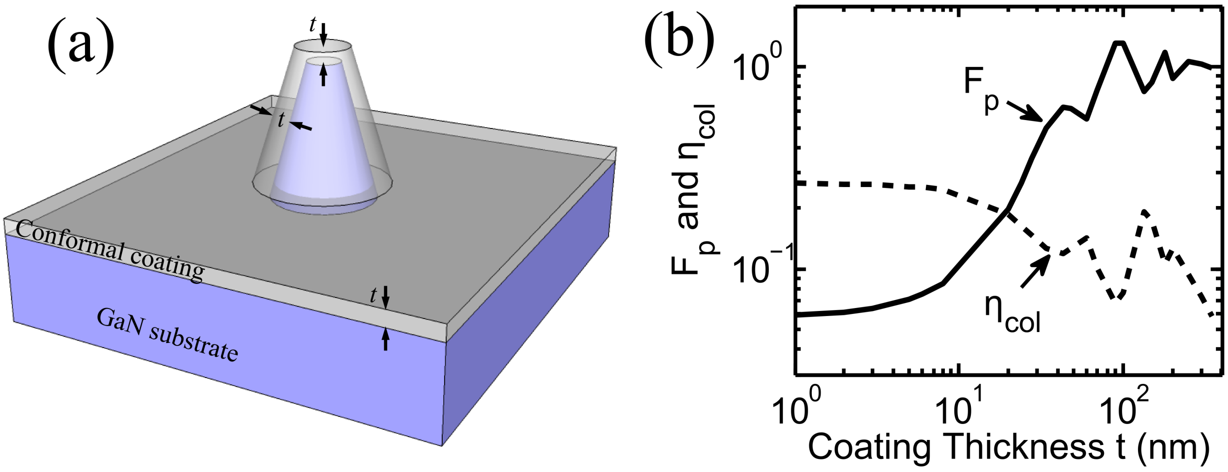


FIG. S4. (a) A schematic plot of conformal coating. (b) The $F_p$, $\eta_{col}$ vs. the coating thickness $t$.

Once we have the $F_p(\vec{p}, r)$ and $\eta_{col}(\vec{p}, r)$ values for all $r$ from 0 to $D/2$, and for both tangential dipole $\vec{p}_\perp$ and radial dipole $\vec{p}_\parallel$, the averaged $F_p$ and $\eta_{col}$ can be calculated as:

$$\overline{F_p} = \frac{4}{D^2}\int_0^{D/2}(F_p(\vec{p}_\perp, r) + F_p(\vec{p}_\parallel, r))r\mathrm{d}r, \tag{S16}$$

$$\overline{\eta_{col}} = \frac{4}{D^2}\int_0^{D/2}(\eta_{col}(\vec{p}_\perp, r) + \eta_{col}(\vec{p}_\parallel, r))r\mathrm{d}r. \tag{S17}$$

The results of $\overline{F_p}$ and $\overline{\eta_{col}}$ are summarized in Fig. 3(a) in the main text.

We note that in Equ. 2-4 of the main text, used to extract $\overline{\gamma_r}$, $\overline{\eta_{int}}$ and $\overline{f_{os}}$, we had to deal with the average-of-product. For example,

$$I \propto P\overline{\eta_{abs}}\,\overline{\eta_{col} f_{os} F_p/\gamma_{tot}}, \tag{S18}$$

in which, $\gamma_{tot}$ includes both $\gamma_r$ ($\propto f_{os}F_p$) and $\gamma_{nr}$. The $P\overline{\eta_{abs}}$ in Equ. S18 is decoupled from the rest of parameters, which reflects that the carrier generation and decay are two independent processes. All parameters in the second average vary with both radial position $r$ and dipole polarization $\vec{p}$. This average-of-product is approximated by the product-of-average: $\overline{\eta_{col}}\,\overline{f_{os}}\,\overline{F_p}\,\overline{1/\gamma_{tot}}$. Due to this approximation, our results on $f_{os}$, $\gamma_r$ and $\eta_{int}$ should be regarded as order-of-magnitude estimations.

## C. Methods to improve $F_p$

A simple way to improve the $F_p$ in NDs in the QD limit, while maintaining the relatively high collection efficiency ($\eta_{col} \sim 15\%$), is conformally coating the sample with GaN, as illustrate in Fig. S4(a). Fig. S4(b) shows the $F_p$ and $\eta_{col}$ of a $D = 30$ nm ND vs. the thickness $t$ of the GaN

coating. As $t$ increases, the $F_p$ is improved by 10 folds to about unity when $t > 70$ nm; the $\eta_{col}$ generally decreases, but has a local maximum at around 150 nm. Therefore, by depositing a 150 nm thick GaN conformally, one can achieve $\sim$ 10-fold $F_p$ enhancement without degrading $\eta_{col}$. More sophisticated methods such as those incorporating tapered nanowires[10] and micro-cavities[11] may improve $\eta_{col}$ and $F_p$ much more.

## REFERENCES


[1] F. Sacconi, M. A. D. Maur, and A. D. Carlo, IEEE Transactions on Electron Devices **59**, 2979 (2012).

[2] S. Chuang and C. Chang, Physical Review B **54**, 2491 (1996).

[3] I. Vurgaftman and J. R. Meyer, Journal of Applied Physics **94**, 3675 (2003).

[4] M. J. Holmes, Y. S. Park, X. Wang, C. C. S. Chan, A. F. Jarjour, R. A. Taylor, J. H. Warner, J. Luo, H. A. R. El-Ella, and R. A. Oliver, Journal of Applied Physics **109**, 063515 (2011).

[5] L. Zhang, T. A. Hill, C.-H. Teng, B. Demory, P.-C. Ku, and H. Deng, ArXiv e-prints (2013), arXiv:1309.4081 [cond-mat.mes-hall].

[6] M. M. Y. Leung, A. B. Djurisic, and E. H. Li, Journal of Applied Physics **84**, 6312 (1998).

[7] L. Novotny and B. Hecht, *Principles of Nano-Optics* (Cambridge University Press, 2006).

[8] W. Lukosz and R. Kunz, Journal of the Optical Society of America **67**, 1607 (1977).

[9] W. Lukosz, Journal of the Optical Society of America **69**, 1495 (1979).

[10] J. Claudon, J. Bleuse, N. Malik, M. Bazin, P. Jaffrennou, N. Gregersen, C. Sauvan, P. Lalanne, and J. Gérard, Nature Photonics **4**, 174 (2010).

[11] O. Gazzano, S. Michaelis de Vasconcellos, C. Arnold, A. Nowak, E. Galopin, I. Sagnes, L. Lanco, A. Lemaître, and P. Senellart, Nature communications **4**, 1425 (2013).
